# Supplementary material for: MAVNet: an Effective Semantic Segmentation Micro-Network for MAV-based Tasks
Source: arXiv:1904.01795 source file (2019-06-08)
Supplement: Supplementary file 1 [file appendix.tex]

\section{Appendix}
\begin{figure*}[t]
  \vspace{3mm}
   \centering
   \includegraphics[width=\linewidth]{{result_images/tunnel_render}}
    \caption{3D volume rendering of the penstock. Pink: corroded, Orange: rivet, Green: water, Pale: coating, Blue: MAV's trajectory}
    \label{fig:intro_image}
    \vspace{-3mm}
\end{figure*}
